# Supplementary material for: Topological extension of the isomorph theory based on the Shannon entropy
Source: arXiv:1901.02772 source file (2019-07-30)
Supplement: Supplementary file 1 [file Supplementary_material_for__Topological_extension_of_the_isomorph_theory_for_scaling_of_particle_dynamics_.pdf]

# Supplementary material for "Topological extension of the isomorph theory based on the Shannon entropy"

Tae Jun Yoon,[1] Min Young Ha,[1] Emanuel A. Lazar,[2] Won Bo Lee,[1, a)] and Youn-Woo Lee[1, b)]
[1)] *School of Chemical and Biological Engineering, Institute of Chemical Processes, Seoul National University, Seoul 08826, Republic of Korea*
[2)] *Department of Mathematics, Bar-Ilan University, Ramat Gan 5290002, Israel*

(Dated: 9 January 2019)

This supplementary material includes the numerical data that can help understand and reproduce the simulation results obtained in the main article.

TABLE S1: Repulsive 8-6 fluids

| $T$ $[K]$ | $\rho$ $[mol/m^3]$ | $p$ $[bar]$ | $U$ $[J/mol]$ | $\Pi_s$ | $s^t_{exc}/k_B$ | $H'$ | $\hat{H}$ | $\sigma_{\hat{H}}$ | $\tilde{D}$ | $\tilde{\eta}$ |
|---|---|---|---|---|---|---|---|---|---|---|
| 318.29 | 2360.30 | 68.57 | 4019.46 | 0.000 | -0.076 | 12.318 | 13.797 | 0.122 | 1.306 | 1.464 |
| 318.29 | 7080.89 | 249.22 | 4140.84 | 0.000 | -0.238 | 12.270 | 13.588 | 0.098 | 0.791 | 0.694 |
| 318.29 | 11801.48 | 506.92 | 4296.23 | 0.000 | -0.414 | 12.182 | 13.415 | 0.147 | 0.534 | 0.516 |
| 318.29 | 16522.07 | 869.09 | 4492.92 | 0.000 | -0.605 | 12.068 | 13.192 | 0.067 | 0.415 | 0.448 |
| 318.29 | 21242.66 | 1375.17 | 4743.56 | 0.001 | -0.811 | 11.916 | 13.008 | 0.138 | 0.341 | 0.460 |
| 318.29 | 25963.25 | 2073.15 | 5059.04 | 0.007 | -1.036 | 11.731 | 12.626 | 0.046 | 0.278 | 0.523 |
| 318.29 | 30683.85 | 3032.25 | 5465.20 | 0.032 | -1.275 | 11.499 | 12.243 | 0.061 | 0.227 | 0.616 |
| 318.29 | 35404.44 | 4328.22 | 5975.50 | 0.118 | -1.533 | 11.220 | 11.916 | 0.072 | 0.192 | 0.762 |
| 318.29 | 40125.03 | 6066.87 | 6620.31 | 0.310 | -1.807 | 10.895 | 11.439 | 0.024 | 0.157 | 0.944 |
| 318.29 | 44845.62 | 8378.24 | 7431.96 | 0.596 | -2.096 | 10.533 | 10.959 | 0.023 | 0.120 | 1.167 |
| 318.29 | 49566.21 | 11393.66 | 8437.23 | 0.844 | -2.400 | 10.131 | 10.487 | 0.054 | 0.102 | 1.444 |
| 318.29 | 54286.81 | 15287.32 | 9675.84 | 0.960 | -2.717 | 9.683 | 9.954 | 0.025 | 0.078 | 1.845 |
| 636.57 | 2360.30 | 135.40 | 8034.02 | 0.000 | -0.064 | 12.318 | 13.795 | 0.079 | 1.632 | 1.572 |
| 636.57 | 7080.89 | 479.33 | 8263.20 | 0.000 | -0.198 | 12.280 | 13.657 | 0.132 | 0.903 | 0.796 |
| 636.57 | 11801.48 | 946.05 | 8543.77 | 0.000 | -0.340 | 12.216 | 13.527 | 0.114 | 0.633 | 0.573 |
| 636.57 | 16522.07 | 1573.60 | 8881.69 | 0.000 | -0.493 | 12.132 | 13.324 | 0.112 | 0.505 | 0.478 |
| 636.57 | 21242.66 | 2411.66 | 9298.53 | 0.000 | -0.656 | 12.021 | 13.129 | 0.109 | 0.410 | 0.449 |
| 636.57 | 25963.25 | 3517.77 | 9808.97 | 0.002 | -0.828 | 11.887 | 12.889 | 0.109 | 0.343 | 0.459 |
| 636.57 | 30683.85 | 4968.45 | 10430.74 | 0.008 | -1.011 | 11.733 | 12.642 | 0.076 | 0.300 | 0.510 |
| 636.57 | 35404.44 | 6855.50 | 11188.76 | 0.026 | -1.203 | 11.549 | 12.352 | 0.062 | 0.246 | 0.589 |
| 636.57 | 40125.03 | 9285.49 | 12103.72 | 0.071 | -1.405 | 11.343 | 12.041 | 0.070 | 0.217 | 0.685 |
| 636.57 | 44845.62 | 12374.70 | 13195.45 | 0.179 | -1.618 | 11.105 | 11.748 | 0.077 | 0.184 | 0.806 |
| 636.57 | 49566.21 | 16281.73 | 14511.33 | 0.362 | -1.839 | 10.831 | 11.371 | 0.059 | 0.159 | 0.961 |
| 636.57 | 54286.81 | 21169.86 | 16075.35 | 0.579 | -2.068 | 10.545 | 10.992 | 0.030 | 0.131 | 1.128 |
| 636.57 | 59007.40 | 27219.49 | 17924.40 | 0.791 | -2.304 | 10.239 | 10.622 | 0.050 | 0.111 | 1.356 |
| 636.57 | 63727.99 | 34634.32 | 20090.51 | 0.915 | -2.546 | 9.904 | 10.224 | 0.031 | 0.091 | 1.614 |
| 636.57 | 68448.58 | 43630.49 | 22611.11 | 0.977 | -2.793 | 9.558 | 9.810 | 0.019 | 0.074 | 1.933 |
| 954.86 | 2360.30 | 201.71 | 12048.08 | 0.000 | -0.057 | 12.322 | 13.917 | 0.200 | 1.863 | 1.822 |
| 954.86 | 7080.89 | 703.00 | 12371.03 | 0.000 | -0.177 | 12.289 | 13.743 | 0.147 | 0.999 | 0.849 |
| 954.86 | 11801.48 | 1366.05 | 12759.90 | 0.000 | -0.303 | 12.239 | 13.522 | 0.052 | 0.693 | 0.618 |
| 954.86 | 16522.07 | 2234.61 | 13224.57 | 0.000 | -0.436 | 12.164 | 13.405 | 0.105 | 0.539 | 0.502 |
| 954.86 | 21242.66 | 3365.06 | 13781.00 | 0.000 | -0.577 | 12.075 | 13.175 | 0.032 | 0.441 | 0.452 |
| 954.86 | 25963.25 | 4824.48 | 14450.37 | 0.001 | -0.725 | 11.970 | 12.960 | 0.053 | 0.372 | 0.453 |
| 954.86 | 30683.85 | 6692.01 | 15244.27 | 0.002 | -0.881 | 11.843 | 12.826 | 0.085 | 0.315 | 0.474 |
| 954.86 | 35404.44 | 9061.70 | 16186.75 | 0.008 | -1.045 | 11.698 | 12.581 | 0.096 | 0.285 | 0.523 |
| 954.86 | 40125.03 | 12051.09 | 17308.39 | 0.026 | -1.215 | 11.533 | 12.353 | 0.075 | 0.240 | 0.585 |
| 954.86 | 44845.62 | 15787.30 | 18633.89 | 0.069 | -1.392 | 11.348 | 12.060 | 0.054 | 0.213 | 0.674 |
| 954.86 | 49566.21 | 20408.31 | 20181.63 | 0.157 | -1.577 | 11.143 | 11.747 | 0.038 | 0.190 | 0.772 |
| 954.86 | 54286.81 | 26097.78 | 22000.02 | 0.305 | -1.767 | 10.914 | 11.459 | 0.025 | 0.170 | 0.894 |
| 954.86 | 59007.40 | 33022.06 | 24104.45 | 0.495 | -1.963 | 10.669 | 11.152 | 0.049 | 0.143 | 1.041 |
| 954.86 | 63727.99 | 41384.37 | 26533.61 | 0.685 | -2.165 | 10.416 | 10.845 | 0.030 | 0.125 | 1.206 |

*Continued on next page*

a) Electronic mail: wblee@snu.ac.kr
b) Electronic mail: ywlee@snu.ac.kr

TABLE S1 – Repulsive 8-6 fluids (continued)

| $T$ $[K]$ | $\rho$ $[mol/m^3]$ | $p$ $[bar]$ | $U$ $[J/mol]$ | $\Pi_s$ | $s^t_{exc}/k_B$ | $H'$ | $\hat{H}$ | $\sigma_{\hat{H}}$ | $\tilde{D}$ | $\tilde{\eta}$ |
|---|---|---|---|---|---|---|---|---|---|---|
| 954.86 | 68448.58 | 51412.10 | 29323.82 | 0.838 | -2.371 | 10.151 | 10.521 | 0.043 | 0.106 | 1.410 |
| 954.86 | 73169.17 | 63322.70 | 32501.51 | 0.932 | -2.582 | 9.851 | 10.179 | 0.026 | 0.087 | 1.640 |
| 954.86 | 77889.76 | 77373.33 | 36107.06 | 0.977 | -2.795 | 9.553 | 9.808 | 0.019 | 0.075 | 1.942 |
| 1273.15 | 2360.30 | 267.50 | 16053.49 | 0.000 | -0.053 | 12.324 | 13.879 | 0.127 | 1.988 | 1.872 |
| 1273.15 | 7080.89 | 923.16 | 16464.89 | 0.000 | -0.162 | 12.294 | 13.667 | 0.071 | 1.074 | 0.867 |
| 1273.15 | 11801.48 | 1775.17 | 16959.55 | 0.000 | -0.277 | 12.247 | 13.625 | 0.135 | 0.720 | 0.634 |
| 1273.15 | 16522.07 | 2871.74 | 17538.49 | 0.000 | -0.398 | 12.187 | 13.442 | 0.040 | 0.572 | 0.515 |
| 1273.15 | 21242.66 | 4274.33 | 18219.91 | 0.000 | -0.525 | 12.108 | 13.365 | 0.169 | 0.495 | 0.459 |
| 1273.15 | 25963.25 | 6055.27 | 19026.92 | 0.000 | -0.658 | 12.021 | 13.150 | 0.123 | 0.397 | 0.443 |
| 1273.15 | 30683.85 | 8296.16 | 19964.72 | 0.001 | -0.798 | 11.906 | 12.918 | 0.061 | 0.343 | 0.460 |
| 1273.15 | 35404.44 | 11105.67 | 21081.13 | 0.004 | -0.943 | 11.787 | 12.788 | 0.134 | 0.311 | 0.489 |
| 1273.15 | 40125.03 | 14586.73 | 22373.80 | 0.015 | -1.095 | 11.640 | 12.491 | 0.107 | 0.264 | 0.536 |
| 1273.15 | 44845.62 | 18883.13 | 23884.79 | 0.033 | -1.252 | 11.496 | 12.263 | 0.082 | 0.243 | 0.606 |
| 1273.15 | 49566.21 | 24134.67 | 25633.96 | 0.076 | -1.415 | 11.321 | 12.005 | 0.053 | 0.218 | 0.684 |
| 1273.15 | 54286.81 | 30520.99 | 27660.25 | 0.177 | -1.582 | 11.124 | 11.766 | 0.059 | 0.190 | 0.773 |
| 1273.15 | 59007.40 | 38206.87 | 29980.69 | 0.296 | -1.754 | 10.935 | 11.510 | 0.062 | 0.165 | 0.880 |
| 1273.15 | 63727.99 | 47415.24 | 32645.22 | 0.451 | -1.931 | 10.715 | 11.192 | 0.030 | 0.143 | 1.011 |
| 1273.15 | 68448.58 | 58335.98 | 35656.30 | 0.624 | -2.112 | 10.491 | 10.910 | 0.024 | 0.130 | 1.156 |
| 1273.15 | 73169.17 | 71226.29 | 39078.01 | 0.790 | -2.296 | 10.245 | 10.627 | 0.032 | 0.110 | 1.325 |
| 1273.15 | 77889.76 | 86301.33 | 42912.84 | 0.892 | -2.485 | 9.998 | 10.316 | 0.018 | 0.101 | 1.523 |
| 1273.15 | 82610.35 | 103837.89 | 47206.17 | 0.958 | -2.677 | 9.732 | 10.009 | 0.018 | 0.079 | 1.765 |
| 1273.15 | 87330.95 | 124122.11 | 51995.14 | 0.983 | -2.871 | 9.461 | 9.698 | 0.020 | 0.070 | 2.026 |
| 1591.44 | 2360.30 | 333.01 | 20051.15 | 0.000 | -0.050 | 12.320 | 13.810 | 0.145 | 2.160 | 2.030 |
| 1591.44 | 7080.89 | 1140.99 | 20559.21 | 0.000 | -0.151 | 12.296 | 13.703 | 0.186 | 1.133 | 0.929 |
| 1591.44 | 11801.48 | 2174.86 | 21141.81 | 0.000 | -0.258 | 12.256 | 13.595 | 0.139 | 0.781 | 0.667 |
| 1591.44 | 16522.07 | 3491.41 | 21820.46 | 0.000 | -0.370 | 12.203 | 13.549 | 0.186 | 0.614 | 0.544 |
| 1591.44 | 21242.66 | 5151.43 | 22620.11 | 0.000 | -0.488 | 12.129 | 13.316 | 0.078 | 0.492 | 0.470 |
| 1591.44 | 25963.25 | 7236.42 | 23555.65 | 0.000 | -0.610 | 12.053 | 13.134 | 0.062 | 0.424 | 0.445 |
| 1591.44 | 30683.85 | 9829.66 | 24637.38 | 0.001 | -0.738 | 11.953 | 12.994 | 0.077 | 0.378 | 0.452 |
| 1591.44 | 35404.44 | 13037.28 | 25893.38 | 0.002 | -0.871 | 11.842 | 12.797 | 0.096 | 0.342 | 0.470 |
| 1591.44 | 40125.03 | 16976.25 | 27347.56 | 0.007 | -1.009 | 11.724 | 12.619 | 0.079 | 0.280 | 0.506 |
| 1591.44 | 44845.62 | 21792.87 | 29030.04 | 0.020 | -1.152 | 11.585 | 12.408 | 0.101 | 0.259 | 0.561 |
| 1591.44 | 49566.21 | 27619.73 | 30953.25 | 0.043 | -1.300 | 11.438 | 12.184 | 0.047 | 0.232 | 0.625 |
| 1591.44 | 54286.81 | 34631.96 | 33160.77 | 0.099 | -1.452 | 11.278 | 11.968 | 0.079 | 0.213 | 0.699 |
| 1591.44 | 59007.40 | 43022.64 | 35684.40 | 0.183 | -1.608 | 11.103 | 11.754 | 0.071 | 0.189 | 0.786 |
| 1591.44 | 63727.99 | 52951.97 | 38519.37 | 0.315 | -1.769 | 10.906 | 11.454 | 0.042 | 0.163 | 0.890 |
| 1591.44 | 68448.58 | 64702.26 | 41751.44 | 0.469 | -1.932 | 10.719 | 11.198 | 0.029 | 0.154 | 1.006 |
| 1591.44 | 73169.17 | 78474.73 | 45381.42 | 0.628 | -2.099 | 10.506 | 10.963 | 0.048 | 0.127 | 1.150 |
| 1591.44 | 77889.76 | 94532.31 | 49454.39 | 0.774 | -2.267 | 10.286 | 10.679 | 0.048 | 0.119 | 1.299 |
| 1591.44 | 82610.35 | 113053.08 | 53950.89 | 0.875 | -2.442 | 10.053 | 10.393 | 0.037 | 0.098 | 1.484 |
| 1591.44 | 87330.95 | 134383.35 | 58946.23 | 0.944 | -2.619 | 9.810 | 10.111 | 0.018 | 0.085 | 1.680 |
| 1591.44 | 92051.54 | 158842.00 | 64485.21 | 0.977 | -2.796 | 9.559 | 9.835 | 0.023 | 0.077 | 1.920 |

TABLE S2: Repulsive 12-6 fluids

| $T$ $[K]$ | $\rho$ $[mol/m^3]$ | $p$ $[bar]$ | $U$ $[J/mol]$ | $\Pi_s$ | $s^t_{exc}/k_B$ | $H'$ | $\hat{H}$ | $\sigma_{\hat{H}}$ | $\tilde{D}$ | $\tilde{\eta}$ |
|---|---|---|---|---|---|---|---|---|---|---|
| 318.29 | 2360.30 | 69.87 | 4009.65 | 0.000 | -0.099 | 12.315 | 13.747 | 0.092 | 1.164 | 1.233 |
| 318.29 | 7080.89 | 263.72 | 4110.11 | 0.000 | -0.315 | 12.243 | 13.554 | 0.121 | 0.644 | 0.640 |
| 318.29 | 11801.48 | 560.25 | 4248.02 | 0.000 | -0.557 | 12.125 | 13.304 | 0.112 | 0.435 | 0.465 |
| 318.29 | 16522.07 | 1007.78 | 4432.37 | 0.001 | -0.831 | 11.941 | 12.969 | 0.128 | 0.319 | 0.447 |
| 318.29 | 21242.66 | 1679.54 | 4680.93 | 0.009 | -1.143 | 11.696 | 12.589 | 0.069 | 0.258 | 0.548 |
| 318.29 | 25963.25 | 2687.35 | 5023.64 | 0.059 | -1.497 | 11.373 | 12.082 | 0.062 | 0.190 | 0.725 |
| 318.29 | 30683.85 | 4188.03 | 5497.16 | 0.273 | -1.900 | 10.939 | 11.548 | 0.062 | 0.156 | 0.998 |
| 318.29 | 35404.44 | 6418.14 | 6153.97 | 0.693 | -2.359 | 10.380 | 10.794 | 0.025 | 0.109 | 1.394 |
| 318.29 | 40125.03 | 9716.44 | 7074.43 | 0.957 | -2.880 | 9.693 | 10.003 | 0.030 | 0.074 | 2.000 |
| 318.29 | 44845.62 | 14557.66 | 8360.36 | 0.999 | -3.465 | 8.858 | 9.050 | 0.021 | 0.043 | 2.944 |
| 318.29 | 2360.30 | 138.15 | 8020.06 | 0.000 | -0.087 | 12.316 | 13.769 | 0.080 | 1.403 | 1.322 |
| 636.57 | 7080.89 | 510.45 | 8225.19 | 0.000 | -0.275 | 12.253 | 13.526 | 0.046 | 0.732 | 0.669 |
| 636.57 | 11801.48 | 1057.56 | 8495.11 | 0.000 | -0.483 | 12.162 | 13.380 | 0.084 | 0.501 | 0.499 |
| 636.57 | 16522.07 | 1850.60 | 8837.66 | 0.000 | -0.716 | 12.012 | 13.127 | 0.094 | 0.380 | 0.438 |
| 636.57 | 21242.66 | 2996.91 | 9294.31 | 0.002 | -0.973 | 11.824 | 12.807 | 0.108 | 0.290 | 0.494 |
| 636.57 | 25963.25 | 4642.97 | 9890.97 | 0.019 | -1.261 | 11.574 | 12.366 | 0.035 | 0.231 | 0.611 |
| 636.57 | 30683.85 | 6989.55 | 10679.70 | 0.097 | -1.581 | 11.256 | 11.960 | 0.077 | 0.181 | 0.784 |
| 636.57 | 35404.44 | 10319.75 | 11723.60 | 0.346 | -1.936 | 10.855 | 11.406 | 0.044 | 0.146 | 1.028 |
| 636.57 | 40125.03 | 15012.50 | 13106.10 | 0.699 | -2.331 | 10.380 | 10.791 | 0.042 | 0.106 | 1.373 |
| 636.57 | 44845.62 | 21599.22 | 14953.96 | 0.946 | -2.764 | 9.783 | 10.089 | 0.033 | 0.079 | 1.863 |
| 636.57 | 49566.21 | 30732.11 | 17386.95 | 0.997 | -3.240 | 9.102 | 9.326 | 0.015 | 0.051 | 2.591 |
| 636.57 | 2360.30 | 205.93 | 12030.21 | 0.000 | -0.081 | 12.322 | 13.845 | 0.111 | 1.543 | 1.432 |
| 636.57 | 7080.89 | 751.01 | 12332.14 | 0.000 | -0.254 | 12.263 | 13.626 | 0.126 | 0.766 | 0.699 |
| 954.86 | 11801.48 | 1531.39 | 12719.27 | 0.000 | -0.444 | 12.176 | 13.392 | 0.120 | 0.540 | 0.506 |
| 954.86 | 16522.07 | 2640.57 | 13214.14 | 0.000 | -0.652 | 12.052 | 13.161 | 0.080 | 0.406 | 0.445 |
| 954.86 | 21242.66 | 4206.04 | 13848.73 | 0.001 | -0.882 | 11.890 | 12.926 | 0.082 | 0.330 | 0.473 |
| 954.86 | 25963.25 | 6396.80 | 14660.47 | 0.011 | -1.137 | 11.675 | 12.524 | 0.042 | 0.258 | 0.556 |
| 954.86 | 30683.85 | 9455.29 | 15714.41 | 0.049 | -1.416 | 11.415 | 12.156 | 0.061 | 0.206 | 0.691 |
| 954.86 | 35404.44 | 13681.63 | 17070.22 | 0.189 | -1.723 | 11.077 | 11.724 | 0.035 | 0.169 | 0.875 |
| 954.86 | 40125.03 | 19511.38 | 18833.04 | 0.458 | -2.059 | 10.698 | 11.196 | 0.030 | 0.130 | 1.128 |
| 954.86 | 44845.62 | 27452.48 | 21094.85 | 0.797 | -2.428 | 10.206 | 10.607 | 0.033 | 0.100 | 1.471 |
| 954.86 | 49566.21 | 38259.79 | 24034.91 | 0.956 | -2.825 | 9.684 | 9.949 | 0.010 | 0.071 | 1.947 |
| 954.86 | 54286.81 | 52721.14 | 27767.71 | 0.997 | -3.258 | 9.046 | 9.260 | 0.015 | 0.050 | 2.646 |
| 954.86 | 2360.30 | 273.41 | 16038.53 | 0.000 | -0.077 | 12.314 | 13.768 | 0.139 | 1.612 | 1.459 |
| 954.86 | 7080.89 | 987.36 | 16435.40 | 0.000 | -0.239 | 12.268 | 13.683 | 0.160 | 0.820 | 0.741 |
| 954.86 | 11801.48 | 1993.09 | 16934.03 | 0.000 | -0.417 | 12.189 | 13.425 | 0.070 | 0.548 | 0.541 |
| 1273.15 | 16522.07 | 3400.61 | 17565.87 | 0.000 | -0.611 | 12.071 | 13.262 | 0.164 | 0.410 | 0.446 |
| 1273.15 | 21242.66 | 5352.30 | 18366.81 | 0.001 | -0.823 | 11.930 | 12.982 | 0.118 | 0.344 | 0.458 |
| 1273.15 | 25963.25 | 8042.47 | 19374.85 | 0.005 | -1.055 | 11.741 | 12.656 | 0.095 | 0.277 | 0.524 |
| 1273.15 | 30683.85 | 11733.96 | 20663.21 | 0.029 | -1.309 | 11.508 | 12.289 | 0.048 | 0.239 | 0.636 |
| 1273.15 | 35404.44 | 16754.88 | 22291.98 | 0.108 | -1.586 | 11.224 | 11.860 | 0.019 | 0.188 | 0.790 |
| 1273.15 | 40125.03 | 23576.45 | 24381.26 | 0.314 | -1.887 | 10.883 | 11.438 | 0.051 | 0.152 | 0.999 |
| 1273.15 | 44845.62 | 32714.08 | 27008.26 | 0.642 | -2.216 | 10.475 | 10.936 | 0.049 | 0.115 | 1.262 |
| 1273.15 | 49566.21 | 44914.90 | 30340.82 | 0.884 | -2.570 | 10.006 | 10.358 | 0.036 | 0.089 | 1.627 |
| 1273.15 | 54286.81 | 61063.53 | 34539.84 | 0.982 | -2.951 | 9.481 | 9.726 | 0.024 | 0.064 | 2.132 |
| 1273.15 | 59007.40 | 82204.11 | 39794.28 | 0.998 | -3.359 | 8.885 | 9.075 | 0.015 | 0.047 | 2.831 |
| 1273.15 | 2360.30 | 340.49 | 20039.36 | 0.000 | -0.074 | 12.317 | 13.837 | 0.231 | 1.682 | 1.551 |
| 1273.15 | 7080.89 | 1220.90 | 20529.51 | 0.000 | -0.228 | 12.277 | 13.654 | 0.118 | 0.861 | 0.766 |
| 1273.15 | 11801.48 | 2445.99 | 21140.46 | 0.000 | -0.396 | 12.201 | 13.453 | 0.083 | 0.587 | 0.553 |
| 1273.15 | 16522.07 | 4138.08 | 21908.95 | 0.000 | -0.578 | 12.091 | 13.210 | 0.042 | 0.442 | 0.461 |
| 1591.44 | 21242.66 | 6455.59 | 22856.31 | 0.001 | -0.778 | 11.953 | 12.986 | 0.063 | 0.349 | 0.454 |
| 1591.44 | 25963.25 | 9619.05 | 24051.18 | 0.004 | -0.995 | 11.787 | 12.741 | 0.060 | 0.290 | 0.502 |
| 1591.44 | 30683.85 | 13893.97 | 25547.12 | 0.019 | -1.231 | 11.578 | 12.402 | 0.066 | 0.250 | 0.601 |
| 1591.44 | 35404.44 | 19650.94 | 27432.17 | 0.076 | -1.487 | 11.325 | 12.031 | 0.089 | 0.198 | 0.733 |
| 1591.44 | 40125.03 | 27350.49 | 29792.33 | 0.239 | -1.765 | 11.013 | 11.597 | 0.033 | 0.170 | 0.911 |
| 1591.44 | 44845.62 | 37559.12 | 32741.15 | 0.486 | -2.066 | 10.652 | 11.156 | 0.044 | 0.129 | 1.139 |
| 1591.44 | 49566.21 | 51036.12 | 36437.17 | 0.779 | -2.389 | 10.248 | 10.620 | 0.044 | 0.108 | 1.437 |
| 1591.44 | 54286.81 | 68703.88 | 41058.10 | 0.948 | -2.734 | 9.769 | 10.083 | 0.033 | 0.078 | 1.830 |
| 1591.44 | 59007.40 | 91569.63 | 46745.21 | 0.993 | -3.105 | 9.242 | 9.487 | 0.033 | 0.058 | 2.360 |
| 1591.44 | 63727.99 | 120972.90 | 53753.04 | 1.000 | -3.498 | 8.656 | 8.836 | 0.018 | 0.041 | 3.147 |

TABLE S3: Repulsive 16-6 fluids

| $T$ $[K]$ | $\rho$ $[mol/m^3]$ | $p$ $[bar]$ | $U$ $[J/mol]$ | $\Pi_s$ | $s^t_{exc}/k_B$ | $H'$ | $\hat{H}$ | $\sigma_{\hat{H}}$ | $\tilde{D}$ | $\tilde{\eta}$ |
|---|---|---|---|---|---|---|---|---|---|---|
| 318.29 | 2360.30 | 70.15 | 4000.63 | 0.000 | -0.107 | 12.310 | 13.773 | 0.144 | 1.116 | 1.249 |
| 318.29 | 7080.89 | 268.51 | 4086.01 | 0.000 | -0.342 | 12.233 | 13.510 | 0.043 | 0.607 | 0.638 |
| 318.29 | 11801.48 | 577.16 | 4199.95 | 0.000 | -0.612 | 12.104 | 13.238 | 0.138 | 0.413 | 0.423 |
| 318.29 | 16522.07 | 1054.73 | 4356.99 | 0.001 | -0.923 | 11.891 | 12.900 | 0.095 | 0.305 | 0.445 |
| 318.29 | 21242.66 | 1791.40 | 4575.53 | 0.015 | -1.283 | 11.618 | 12.428 | 0.063 | 0.227 | 0.588 |
| 318.29 | 25963.25 | 2928.20 | 4884.32 | 0.111 | -1.703 | 11.227 | 11.911 | 0.064 | 0.165 | 0.841 |
| 318.29 | 30683.85 | 4675.38 | 5318.94 | 0.458 | -2.198 | 10.684 | 11.206 | 0.043 | 0.121 | 1.207 |
| 318.29 | 35404.44 | 7379.30 | 5951.22 | 0.885 | -2.782 | 9.987 | 10.336 | 0.024 | 0.079 | 1.799 |
| 318.29 | 40125.03 | 11579.51 | 6881.51 | 0.997 | -3.470 | 9.071 | 9.291 | 0.017 | 0.048 | 2.772 |
| 636.57 | 2360.30 | 139.14 | 8005.78 | 0.000 | -0.098 | 12.319 | 13.739 | 0.082 | 1.272 | 1.287 |
| 636.57 | 7080.89 | 522.19 | 8180.45 | 0.000 | -0.309 | 12.248 | 13.586 | 0.093 | 0.678 | 0.651 |
| 636.57 | 11801.48 | 1100.38 | 8411.27 | 0.000 | -0.549 | 12.131 | 13.305 | 0.093 | 0.456 | 0.464 |
| 636.57 | 16522.07 | 1964.23 | 8721.08 | 0.001 | -0.819 | 11.961 | 13.076 | 0.119 | 0.355 | 0.430 |
| 636.57 | 21242.66 | 3251.91 | 9134.25 | 0.007 | -1.128 | 11.728 | 12.605 | 0.057 | 0.268 | 0.534 |
| 636.57 | 25963.25 | 5163.01 | 9694.47 | 0.048 | -1.482 | 11.411 | 12.169 | 0.071 | 0.199 | 0.709 |
| 636.57 | 30683.85 | 8005.55 | 10471.02 | 0.230 | -1.885 | 11.005 | 11.611 | 0.085 | 0.149 | 0.971 |
| 636.57 | 35404.44 | 12210.58 | 11531.15 | 0.633 | -2.352 | 10.465 | 10.928 | 0.049 | 0.106 | 1.362 |
| 636.57 | 40125.03 | 18443.29 | 13022.51 | 0.943 | -2.889 | 9.777 | 10.093 | 0.024 | 0.075 | 1.960 |
| 636.57 | 44845.62 | 27672.37 | 15116.24 | 0.999 | -3.505 | 8.929 | 9.131 | 0.022 | 0.046 | 2.908 |
| 954.86 | 2360.30 | 207.68 | 12012.15 | 0.000 | -0.092 | 12.316 | 13.780 | 0.140 | 1.398 | 1.435 |
| 954.86 | 7080.89 | 770.48 | 12273.00 | 0.000 | -0.291 | 12.251 | 13.555 | 0.108 | 0.699 | 0.678 |
| 954.86 | 11801.48 | 1602.91 | 12614.73 | 0.000 | -0.513 | 12.145 | 13.299 | 0.040 | 0.493 | 0.480 |
| 954.86 | 16522.07 | 2824.30 | 13063.43 | 0.000 | -0.762 | 11.995 | 13.089 | 0.103 | 0.349 | 0.429 |
| 954.86 | 21242.66 | 4604.04 | 13655.99 | 0.004 | -1.044 | 11.794 | 12.741 | 0.109 | 0.286 | 0.501 |
| 954.86 | 25963.25 | 7201.68 | 14444.74 | 0.027 | -1.362 | 11.524 | 12.271 | 0.057 | 0.220 | 0.646 |
| 954.86 | 30683.85 | 10965.50 | 15507.89 | 0.144 | -1.722 | 11.162 | 11.832 | 0.063 | 0.168 | 0.865 |
| 954.86 | 35404.44 | 16410.86 | 16930.79 | 0.455 | -2.133 | 10.700 | 11.207 | 0.050 | 0.128 | 1.168 |
| 954.86 | 40125.03 | 24294.98 | 18876.96 | 0.827 | -2.597 | 10.132 | 10.494 | 0.019 | 0.090 | 1.616 |
| 954.86 | 44845.62 | 35653.97 | 21525.66 | 0.987 | -3.127 | 9.413 | 9.674 | 0.025 | 0.063 | 2.289 |
| 954.86 | 49566.21 | 51992.28 | 25160.96 | 1.000 | -3.723 | 8.566 | 8.732 | 0.015 | 0.036 | 3.402 |
| 1273.15 | 2360.30 | 275.80 | 16017.18 | 0.000 | -0.088 | 12.313 | 13.824 | 0.150 | 1.479 | 1.422 |
| 1273.15 | 7080.89 | 1015.00 | 16360.28 | 0.000 | -0.277 | 12.260 | 13.590 | 0.069 | 0.737 | 0.697 |
| 1273.15 | 11801.48 | 2092.77 | 16811.99 | 0.000 | -0.487 | 12.162 | 13.350 | 0.072 | 0.484 | 0.496 |
| 1273.15 | 16522.07 | 3653.13 | 17399.12 | 0.000 | -0.722 | 12.020 | 13.180 | 0.121 | 0.374 | 0.425 |
| 1273.15 | 21242.66 | 5898.23 | 18156.52 | 0.003 | -0.985 | 11.826 | 12.831 | 0.116 | 0.287 | 0.489 |
| 1273.15 | 25963.25 | 9113.65 | 19152.74 | 0.020 | -1.281 | 11.583 | 12.401 | 0.085 | 0.230 | 0.614 |
| 1273.15 | 30683.85 | 13713.68 | 20473.77 | 0.098 | -1.613 | 11.261 | 11.920 | 0.030 | 0.195 | 0.796 |
| 1273.15 | 35404.44 | 20270.95 | 22223.73 | 0.330 | -1.988 | 10.857 | 11.413 | 0.058 | 0.140 | 1.056 |
| 1273.15 | 40125.03 | 29598.12 | 24561.23 | 0.728 | -2.409 | 10.347 | 10.757 | 0.027 | 0.106 | 1.431 |
| 1273.15 | 44845.62 | 42816.46 | 27689.95 | 0.954 | -2.885 | 9.730 | 10.040 | 0.024 | 0.069 | 1.965 |
| 1273.15 | 49566.21 | 61491.25 | 31898.68 | 0.998 | -3.419 | 8.987 | 9.188 | 0.015 | 0.051 | 2.783 |
| 1273.15 | 54286.81 | 87748.47 | 37536.17 | 1.000 | -4.015 | 8.118 | 8.249 | 0.011 | 0.026 | 4.202 |
| 1591.44 | 2360.30 | 343.70 | 20021.98 | 0.000 | -0.085 | 12.318 | 13.797 | 0.126 | 1.528 | 1.394 |
| 1591.44 | 7080.89 | 1257.22 | 20449.87 | 0.000 | -0.267 | 12.264 | 13.588 | 0.069 | 0.756 | 0.690 |
| 1591.44 | 11801.48 | 2574.54 | 21006.17 | 0.000 | -0.468 | 12.175 | 13.419 | 0.130 | 0.498 | 0.516 |
| 1591.44 | 16522.07 | 4461.39 | 21718.73 | 0.000 | -0.692 | 12.038 | 13.173 | 0.153 | 0.385 | 0.434 |
| 1591.44 | 21242.66 | 7145.81 | 22634.02 | 0.002 | -0.942 | 11.861 | 12.866 | 0.099 | 0.301 | 0.476 |
| 1591.44 | 25963.25 | 10954.30 | 23829.60 | 0.013 | -1.221 | 11.630 | 12.478 | 0.057 | 0.253 | 0.585 |
| 1591.44 | 30683.85 | 16328.50 | 25385.04 | 0.073 | -1.534 | 11.331 | 12.045 | 0.038 | 0.196 | 0.750 |
| 1591.44 | 35404.44 | 23900.41 | 27428.46 | 0.255 | -1.884 | 10.966 | 11.537 | 0.054 | 0.147 | 0.980 |
| 1591.44 | 40125.03 | 34516.60 | 30107.24 | 0.604 | -2.276 | 10.507 | 10.960 | 0.028 | 0.110 | 1.309 |
| 1591.44 | 44845.62 | 49443.61 | 33694.07 | 0.904 | -2.713 | 9.952 | 10.284 | 0.038 | 0.082 | 1.755 |
| 1591.44 | 49566.21 | 70183.96 | 38384.02 | 0.993 | -3.205 | 9.273 | 9.522 | 0.027 | 0.058 | 2.419 |
| 1591.44 | 54286.81 | 99014.13 | 44618.21 | 1.000 | -3.751 | 8.475 | 8.645 | 0.009 | 0.033 | 3.523 |

TABLE S4: Repulsive 20-6 fluids

| $T$ $[K]$ | $\rho$ $[mol/m^3]$ | $p$ $[bar]$ | $U$ $[J/mol]$ | $\Pi_s$ | $s^t_{exc}/k_B$ | $H'$ | $\hat{H}$ | $\sigma_{\hat{H}}$ | $\tilde{D}$ | $\tilde{\eta}$ |
|---|---|---|---|---|---|---|---|---|---|---|
| 318.29 | 2360.30 | 70.32 | 3996.05 | 0.000 | -0.111 | 12.314 | 13.731 | 0.058 | 1.090 | 1.171 |
| 318.29 | 7080.89 | 270.25 | 4067.67 | 0.000 | -0.357 | 12.235 | 13.563 | 0.141 | 0.573 | 0.629 |
| 318.29 | 11801.48 | 584.72 | 4164.02 | 0.000 | -0.642 | 12.093 | 13.268 | 0.094 | 0.388 | 0.387 |
| 318.29 | 16522.07 | 1075.92 | 4300.50 | 0.002 | -0.972 | 11.872 | 12.849 | 0.063 | 0.289 | 0.434 |
| 318.29 | 21242.66 | 1842.25 | 4490.12 | 0.018 | -1.359 | 11.571 | 12.400 | 0.073 | 0.220 | 0.602 |
| 318.29 | 25963.25 | 3039.45 | 4758.44 | 0.144 | -1.819 | 11.149 | 11.784 | 0.033 | 0.162 | 0.884 |
| 318.29 | 30683.85 | 4924.00 | 5152.29 | 0.559 | -2.370 | 10.573 | 11.026 | 0.029 | 0.112 | 1.328 |
| 318.29 | 35404.44 | 7894.99 | 5728.48 | 0.946 | -3.035 | 9.777 | 10.100 | 0.027 | 0.065 | 2.052 |
| 636.57 | 2360.30 | 139.63 | 7997.42 | 0.000 | -0.103 | 12.318 | 13.808 | 0.083 | 1.255 | 1.298 |
| 636.57 | 7080.89 | 528.35 | 8145.07 | 0.000 | -0.329 | 12.245 | 13.611 | 0.173 | 0.655 | 0.635 |
| 636.57 | 11801.48 | 1122.42 | 8346.14 | 0.000 | -0.586 | 12.116 | 13.290 | 0.089 | 0.434 | 0.438 |
| 636.57 | 16522.07 | 2025.25 | 8618.94 | 0.001 | -0.881 | 11.934 | 13.015 | 0.118 | 0.314 | 0.424 |
| 636.57 | 21242.66 | 3393.01 | 8987.30 | 0.010 | -1.222 | 11.672 | 12.538 | 0.081 | 0.250 | 0.557 |
| 636.57 | 25963.25 | 5463.36 | 9501.27 | 0.073 | -1.617 | 11.328 | 12.001 | 0.040 | 0.188 | 0.769 |
| 636.57 | 30683.85 | 8607.51 | 10218.78 | 0.338 | -2.080 | 10.850 | 11.398 | 0.049 | 0.136 | 1.096 |
| 636.57 | 35404.44 | 13371.33 | 11228.03 | 0.794 | -2.628 | 10.212 | 10.596 | 0.029 | 0.100 | 1.597 |
| 636.57 | 40125.03 | 20685.85 | 12691.44 | 0.987 | -3.273 | 9.387 | 9.651 | 0.021 | 0.058 | 2.399 |
| 954.86 | 2360.30 | 208.43 | 11992.41 | 0.000 | -0.098 | 12.315 | 13.783 | 0.111 | 1.347 | 1.287 |
| 954.86 | 7080.89 | 781.02 | 12225.61 | 0.000 | -0.311 | 12.247 | 13.635 | 0.127 | 0.693 | 0.654 |
| 954.86 | 11801.48 | 1642.56 | 12527.39 | 0.000 | -0.553 | 12.138 | 13.332 | 0.101 | 0.446 | 0.455 |
| 954.86 | 16522.07 | 2928.62 | 12926.74 | 0.001 | -0.828 | 11.966 | 12.983 | 0.088 | 0.333 | 0.420 |
| 954.86 | 21242.66 | 4842.65 | 13467.41 | 0.005 | -1.143 | 11.726 | 12.623 | 0.091 | 0.262 | 0.529 |
| 954.86 | 25963.25 | 7689.94 | 14196.62 | 0.046 | -1.505 | 11.413 | 12.197 | 0.080 | 0.199 | 0.712 |
| 954.86 | 30683.85 | 11913.50 | 15195.75 | 0.235 | -1.924 | 11.000 | 11.583 | 0.041 | 0.146 | 0.984 |
| 954.86 | 35404.44 | 18211.94 | 16587.05 | 0.641 | -2.411 | 10.458 | 10.886 | 0.035 | 0.105 | 1.390 |
| 954.86 | 40125.03 | 27619.68 | 18541.17 | 0.949 | -2.980 | 9.736 | 10.062 | 0.021 | 0.072 | 2.015 |
| 954.86 | 44845.62 | 41693.20 | 21300.44 | 0.999 | -3.646 | 8.835 | 9.037 | 0.022 | 0.041 | 3.041 |
| 1273.15 | 2360.30 | 277.11 | 15994.88 | 0.000 | -0.095 | 12.315 | 13.822 | 0.161 | 1.417 | 1.332 |
| 1273.15 | 7080.89 | 1030.94 | 16299.37 | 0.000 | -0.300 | 12.254 | 13.558 | 0.076 | 0.685 | 0.660 |
| 1273.15 | 11801.48 | 2151.29 | 16702.21 | 0.000 | -0.531 | 12.142 | 13.374 | 0.124 | 0.472 | 0.484 |
| 1273.15 | 16522.07 | 3802.69 | 17226.28 | 0.000 | -0.793 | 11.988 | 13.054 | 0.088 | 0.342 | 0.414 |
| 1273.15 | 21242.66 | 6231.49 | 17926.45 | 0.004 | -1.090 | 11.774 | 12.714 | 0.089 | 0.279 | 0.502 |
| 1273.15 | 25963.25 | 9790.94 | 18859.85 | 0.035 | -1.430 | 11.479 | 12.276 | 0.086 | 0.209 | 0.668 |
| 1273.15 | 30683.85 | 15009.91 | 20117.50 | 0.182 | -1.821 | 11.098 | 11.759 | 0.070 | 0.154 | 0.906 |
| 1273.15 | 35404.44 | 22680.49 | 21851.98 | 0.536 | -2.270 | 10.599 | 11.077 | 0.037 | 0.114 | 1.261 |
| 1273.15 | 40125.03 | 33954.71 | 24244.95 | 0.897 | -2.791 | 9.971 | 10.319 | 0.032 | 0.081 | 1.796 |
| 1273.15 | 44845.62 | 50537.67 | 27557.39 | 0.995 | -3.396 | 9.169 | 9.382 | 0.016 | 0.052 | 2.632 |
| 1591.44 | 2360.30 | 345.48 | 19996.75 | 0.000 | -0.092 | 12.317 | 13.880 | 0.173 | 1.514 | 1.420 |
| 1591.44 | 7080.89 | 1278.30 | 20377.05 | 0.000 | -0.291 | 12.257 | 13.554 | 0.055 | 0.714 | 0.683 |
| 1591.44 | 11801.48 | 2650.07 | 20866.82 | 0.000 | -0.514 | 12.153 | 13.308 | 0.044 | 0.490 | 0.483 |
| 1591.44 | 16522.07 | 4658.31 | 21514.89 | 0.000 | -0.765 | 12.000 | 13.092 | 0.105 | 0.358 | 0.417 |
| 1591.44 | 21242.66 | 7577.56 | 22368.33 | 0.004 | -1.050 | 11.795 | 12.715 | 0.056 | 0.274 | 0.494 |
| 1591.44 | 25963.25 | 11819.30 | 23499.21 | 0.027 | -1.373 | 11.525 | 12.298 | 0.049 | 0.213 | 0.638 |
| 1591.44 | 30683.85 | 17975.40 | 25012.48 | 0.136 | -1.743 | 11.168 | 11.795 | 0.017 | 0.167 | 0.865 |
| 1591.44 | 35404.44 | 26903.86 | 27046.74 | 0.452 | -2.166 | 10.716 | 11.220 | 0.033 | 0.127 | 1.182 |
| 1591.44 | 40125.03 | 39881.55 | 29834.42 | 0.831 | -2.652 | 10.131 | 10.544 | 0.033 | 0.088 | 1.646 |
| 1591.44 | 44845.62 | 58714.47 | 33639.26 | 0.987 | -3.215 | 9.397 | 9.649 | 0.023 | 0.055 | 2.364 |
| 1591.44 | 49566.21 | 86158.84 | 38913.65 | 1.000 | -3.861 | 8.503 | 8.650 | 0.013 | 0.035 | 3.561 |

TABLE S5: Repulsive 24-6 fluids

| $T$ [$K$] | $\rho$ [$mol/m^3$] | $p$ [$bar$] | $U$ [$J/mol$] | $\Pi_s$ | $s^t_{exc}/k_B$ | $H'$ | $\hat{H}$ | $\sigma_{\hat{H}}$ | $\tilde{D}$ | $\tilde{\eta}$ |
|---|---|---|---|---|---|---|---|---|---|---|
| 318.29 | 2360.30 | 70.39 | 3992.62 | 0.000 | -0.114 | 12.312 | 13.808 | 0.148 | 1.113 | 1.210 |
| 318.29 | 7080.89 | 271.21 | 4054.35 | 0.000 | -0.366 | 12.231 | 13.538 | 0.097 | 0.587 | 0.618 |
| 318.29 | 11801.48 | 589.16 | 4140.27 | 0.000 | -0.659 | 12.087 | 13.166 | 0.036 | 0.390 | 0.356 |
| 318.29 | 16522.07 | 1087.36 | 4257.87 | 0.002 | -1.003 | 11.865 | 12.881 | 0.095 | 0.281 | 0.416 |
| 318.29 | 21242.66 | 1870.16 | 4423.39 | 0.023 | -1.408 | 11.556 | 12.371 | 0.093 | 0.206 | 0.607 |
| 318.29 | 25963.25 | 3102.72 | 4662.96 | 0.170 | -1.893 | 11.109 | 11.725 | 0.031 | 0.149 | 0.911 |
| 318.29 | 30683.85 | 5056.77 | 5011.16 | 0.616 | -2.482 | 10.498 | 10.958 | 0.047 | 0.101 | 1.389 |
| 318.29 | 35404.44 | 8189.96 | 5533.16 | 0.967 | -3.201 | 9.645 | 9.945 | 0.034 | 0.061 | 2.168 |
| 636.57 | 2360.30 | 139.97 | 7989.11 | 0.000 | -0.107 | 12.313 | 13.789 | 0.089 | 1.231 | 1.281 |
| 636.57 | 7080.89 | 531.51 | 8120.23 | 0.000 | -0.341 | 12.242 | 13.521 | 0.078 | 0.649 | 0.634 |
| 636.57 | 11801.48 | 1136.31 | 8297.96 | 0.000 | -0.610 | 12.111 | 13.301 | 0.102 | 0.423 | 0.402 |
| 636.57 | 16522.07 | 2062.25 | 8539.33 | 0.001 | -0.921 | 11.913 | 12.921 | 0.075 | 0.302 | 0.409 |
| 636.57 | 21242.66 | 3480.56 | 8871.73 | 0.012 | -1.283 | 11.642 | 12.491 | 0.101 | 0.235 | 0.560 |
| 636.57 | 25963.25 | 5647.93 | 9330.05 | 0.092 | -1.710 | 11.263 | 11.968 | 0.080 | 0.171 | 0.809 |
| 636.57 | 30683.85 | 8989.77 | 9988.40 | 0.426 | -2.214 | 10.745 | 11.227 | 0.031 | 0.121 | 1.179 |
| 636.57 | 35404.44 | 14160.78 | 10934.30 | 0.861 | -2.820 | 10.052 | 10.416 | 0.033 | 0.078 | 1.750 |
| 636.57 | 40125.03 | 22222.68 | 12320.98 | 0.996 | -3.550 | 9.129 | 9.353 | 0.029 | 0.045 | 2.735 |
| 954.86 | 2360.30 | 208.97 | 11982.48 | 0.000 | -0.102 | 12.319 | 13.778 | 0.145 | 1.352 | 1.265 |
| 954.86 | 7080.89 | 787.91 | 12184.59 | 0.000 | -0.326 | 12.251 | 13.612 | 0.127 | 0.638 | 0.643 |
| 954.86 | 11801.48 | 1667.93 | 12458.51 | 0.000 | -0.580 | 12.124 | 13.310 | 0.099 | 0.455 | 0.430 |
| 954.86 | 16522.07 | 2995.26 | 12812.12 | 0.001 | -0.874 | 11.946 | 12.925 | 0.026 | 0.318 | 0.404 |
| 954.86 | 21242.66 | 4999.51 | 13305.86 | 0.007 | -1.212 | 11.693 | 12.566 | 0.088 | 0.237 | 0.535 |
| 954.86 | 25963.25 | 8007.65 | 13968.12 | 0.067 | -1.607 | 11.347 | 12.102 | 0.070 | 0.187 | 0.749 |
| 954.86 | 30683.85 | 12557.57 | 14899.86 | 0.323 | -2.069 | 10.885 | 11.466 | 0.061 | 0.127 | 1.063 |
| 954.86 | 35404.44 | 19476.22 | 16220.68 | 0.759 | -2.616 | 10.276 | 10.671 | 0.035 | 0.094 | 1.558 |
| 954.86 | 40125.03 | 30031.17 | 18108.71 | 0.982 | -3.268 | 9.471 | 9.730 | 0.021 | 0.058 | 2.336 |
| 1273.15 | 2360.30 | 277.98 | 15982.09 | 0.000 | -0.099 | 12.315 | 13.772 | 0.177 | 1.344 | 1.349 |
| 1273.15 | 7080.89 | 1040.88 | 16250.98 | 0.000 | -0.316 | 12.250 | 13.651 | 0.110 | 0.669 | 0.674 |
| 1273.15 | 11801.48 | 2188.32 | 16606.42 | 0.000 | -0.561 | 12.135 | 13.285 | 0.051 | 0.456 | 0.445 |
| 1273.15 | 16522.07 | 3903.25 | 17086.58 | 0.000 | -0.841 | 11.963 | 12.959 | 0.073 | 0.336 | 0.400 |
| 1273.15 | 21242.66 | 6455.09 | 17718.12 | 0.006 | -1.164 | 11.724 | 12.667 | 0.091 | 0.256 | 0.513 |
| 1273.15 | 25963.25 | 10264.78 | 18592.56 | 0.048 | -1.536 | 11.408 | 12.154 | 0.070 | 0.193 | 0.713 |
| 1273.15 | 30683.85 | 15929.90 | 19775.50 | 0.242 | -1.971 | 10.985 | 11.580 | 0.049 | 0.146 | 1.000 |
| 1273.15 | 35404.44 | 24425.49 | 21437.11 | 0.665 | -2.481 | 10.416 | 10.848 | 0.042 | 0.103 | 1.429 |
| 1273.15 | 40125.03 | 37216.23 | 23773.39 | 0.962 | -3.084 | 9.686 | 9.968 | 0.017 | 0.065 | 2.096 |
| 1591.44 | 2360.30 | 346.60 | 19975.20 | 0.000 | -0.097 | 12.312 | 13.768 | 0.076 | 1.421 | 1.359 |
| 1591.44 | 7080.89 | 1292.52 | 20314.52 | 0.000 | -0.308 | 12.255 | 13.547 | 0.033 | 0.680 | 0.666 |
| 1591.44 | 11801.48 | 2702.63 | 20763.79 | 0.000 | -0.546 | 12.141 | 13.369 | 0.151 | 0.465 | 0.453 |
| 1591.44 | 16522.07 | 4791.08 | 21348.86 | 0.001 | -0.817 | 11.974 | 13.074 | 0.082 | 0.349 | 0.402 |
| 1591.44 | 21242.66 | 7872.58 | 22126.60 | 0.005 | -1.127 | 11.762 | 12.653 | 0.033 | 0.255 | 0.503 |
| 1591.44 | 25963.25 | 12429.54 | 23187.49 | 0.037 | -1.483 | 11.455 | 12.238 | 0.117 | 0.204 | 0.682 |
| 1591.44 | 30683.85 | 19151.84 | 24612.01 | 0.197 | -1.897 | 11.058 | 11.713 | 0.066 | 0.158 | 0.950 |
| 1591.44 | 35404.44 | 29115.22 | 26585.82 | 0.590 | -2.379 | 10.527 | 10.979 | 0.024 | 0.108 | 1.344 |
| 1591.44 | 40125.03 | 43964.09 | 29345.58 | 0.930 | -2.945 | 9.843 | 10.184 | 0.041 | 0.077 | 1.937 |
| 1591.44 | 44845.62 | 66121.44 | 33212.12 | 0.998 | -3.614 | 8.981 | 9.174 | 0.023 | 0.045 | 2.891 |
